# Supplementary material for: Differentiable Neural Architecture Search for Extremely Lightweight Image Super-Resolution
Source: arXiv:2105.03939 source file (2022-12-19)
Supplement: Supplementary file 1 [file 7.appendix.tex]

\newpage
\onecolumn

\section{More Visual Comparison Results}
More visual comparison results show that our DLSR model has superior performance compared with other lightweight SR models on image details. In Figure \ref{Fig.more_X4} and Figure \ref{Fig.more_X42}, our method reconstructs the stripe-like and lattice-like image details on the buildings without distortion.

\begin{figure*}[ht]
\centering
\subfloat[HR]{
\begin{minipage}[t]{0.15\linewidth}
\centering
\label{Fig.more_x4_hr}
\includegraphics[width=1.1in,height=0.8in]{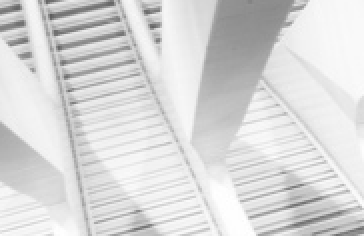}\\
\includegraphics[width=1.1in]{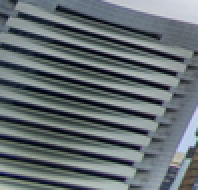}\\
\includegraphics[width=1.1in,height=0.8in]{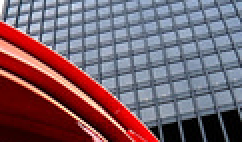}\\

\end{minipage}
}
\subfloat[Bicubic]{
\begin{minipage}[t]{0.15\linewidth}
\centering
\label{Fig.more_x4_bic}
\includegraphics[width=1.1in,height=0.8in]{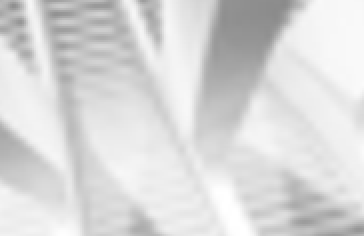}\\
\includegraphics[width=1.1in]{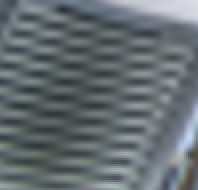}\\
\includegraphics[width=1.1in,height=0.8in]{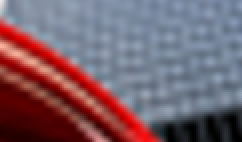}\\

\end{minipage}
}
\subfloat[CARN-M]{
\begin{minipage}[t]{0.15\linewidth}
\centering
\label{Fig.more_x4_carn-m}
\includegraphics[width=1.1in,height=0.8in]{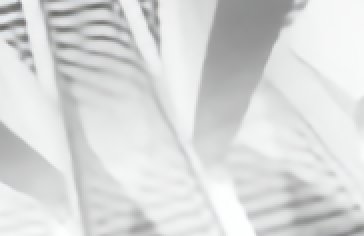}\\
\includegraphics[width=1.1in]{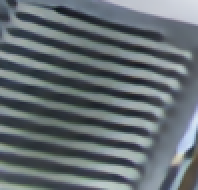}\\
\includegraphics[width=1.1in,height=0.8in]{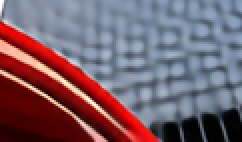}\\

\end{minipage}
}
\subfloat[RFDN]{
\begin{minipage}[t]{0.15\linewidth}
\centering
\label{Fig.more_x4_RFDN}
\includegraphics[width=1.1in,height=0.8in]{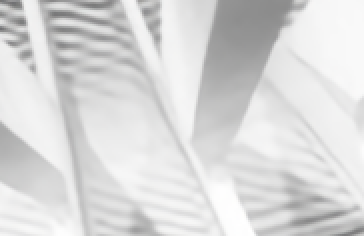}\\
\includegraphics[width=1.1in]{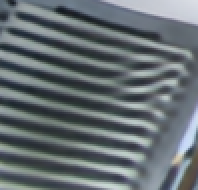}\\
\includegraphics[width=1.1in,height=0.8in]{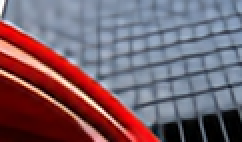}\\

\end{minipage}
}
\subfloat[PAN]{
\begin{minipage}[t]{0.15\linewidth}
\centering
\label{Fig.more_x4_PAN}
\includegraphics[width=1.1in,height=0.8in]{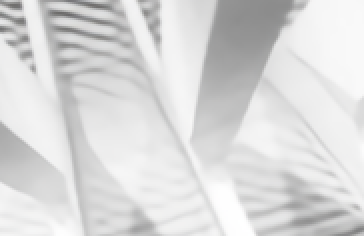}\\
\includegraphics[width=1.1in]{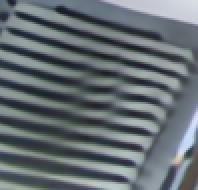}\\
\includegraphics[width=1.1in,height=0.8in]{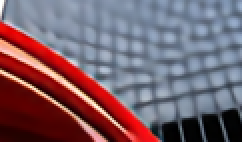}\\

\end{minipage}
}
\subfloat[Ours]{
\begin{minipage}[t]{0.15\linewidth}
\centering
\label{Fig.more_x4_OURS}
\includegraphics[width=1.1in,height=0.8in]{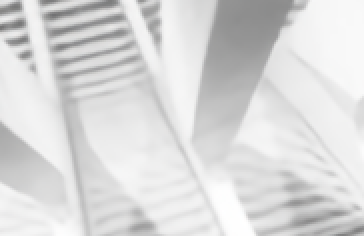}\\
\includegraphics[width=1.1in]{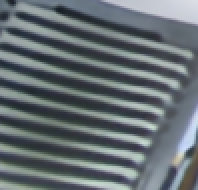}\\
\includegraphics[width=1.1in,height=0.8in]{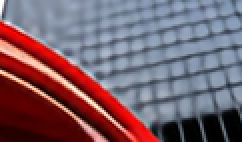}\\

\end{minipage}
}
\caption{Visual comparisons among SOTA lightweight models in $\times 4$ image super-resolution. The test image patches are from Urban100. Note that the results of RFDN are based on our test with the pre-trained model which is officially released by the authors. Our method shows better reconstruction performance and less deformation on image details.}
\label{Fig.more_X4}
%\vspace{-0.6cm}
\centering
\subfloat[HR]{
\begin{minipage}[t]{0.15\linewidth}
\centering
\label{Fig.more_x4_hr2}

\includegraphics[width=1.1in,height=1.2in]{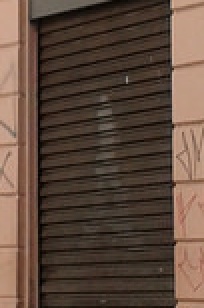}\\
\includegraphics[width=1.1in,height=0.8in]{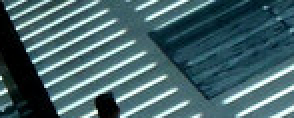}\\
\includegraphics[width=1.1in,height=0.8in]{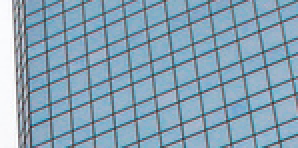}
\end{minipage}
}
\subfloat[Bicubic]{
\begin{minipage}[t]{0.15\linewidth}
\centering
\label{Fig.more_x4_bic2}

\includegraphics[width=1.1in,height=1.2in]{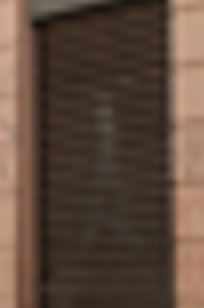}\\
\includegraphics[width=1.1in,height=0.8in]{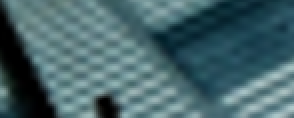}\\
\includegraphics[width=1.1in,height=0.8in]{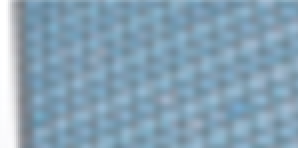}
\end{minipage}
}
\subfloat[CARN-M]{
\begin{minipage}[t]{0.15\linewidth}
\centering
\label{Fig.more_x4_carn-m2}

\includegraphics[width=1.1in,height=1.2in]{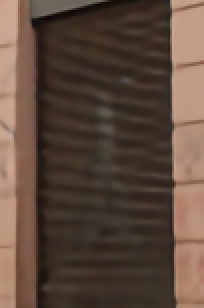}\\
\includegraphics[width=1.1in,height=0.8in]{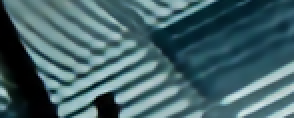}\\
\includegraphics[width=1.1in,height=0.8in]{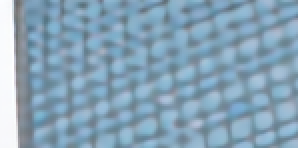}
\end{minipage}
}
\subfloat[RFDN]{
\begin{minipage}[t]{0.15\linewidth}
\centering
\label{Fig.more_x4_RFDN2}

\includegraphics[width=1.1in,height=1.2in]{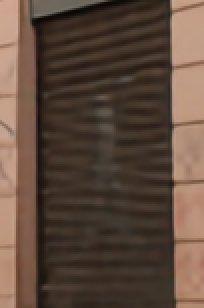}\\
\includegraphics[width=1.1in,height=0.8in]{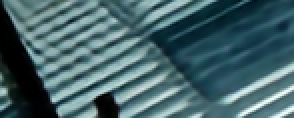}\\
\includegraphics[width=1.1in,height=0.8in]{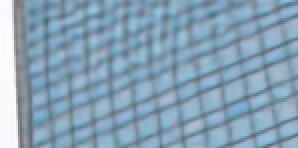}
\end{minipage}
}
\subfloat[PAN]{
\begin{minipage}[t]{0.15\linewidth}
\centering
\label{Fig.more_x4_PAN2}

\includegraphics[width=1.1in,height=1.2in]{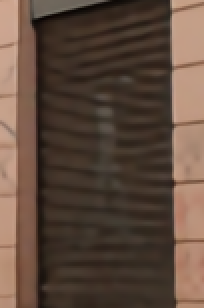}\\
\includegraphics[width=1.1in,height=0.8in]{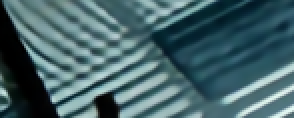}\\
\includegraphics[width=1.1in,height=0.8in]{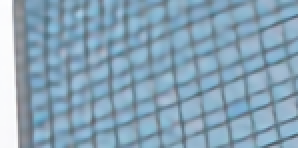}\\
\end{minipage}
}
\subfloat[Ours]{
\begin{minipage}[t]{0.15\linewidth}
\centering
\label{Fig.more_x4_OURS2}

\includegraphics[width=1.1in,height=1.2in]{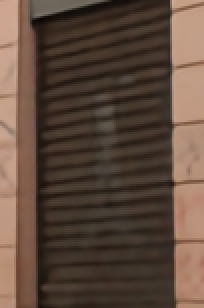}\\
\includegraphics[width=1.1in,height=0.8in]{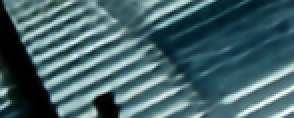}\\
\includegraphics[width=1.1in,height=0.8in]{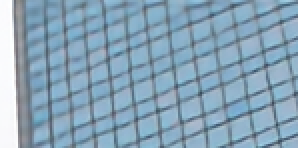}
\end{minipage}
}
\caption{Visual comparisons among SOTA lightweight models in $\times 4$ image super-resolution. The test image patches are from Urban100. Note that the results of RFDN are based on our test with the pre-trained model which is officially released by the authors. Our method shows better reconstruction performance and less deformation on image details.}
\label{Fig.more_X42}
%\vspace{-0.1cm}
\end{figure*}
